# Supplementary material for: Model-independent search for CP violation in D0 to K-K+pi-pi+ and D0 to pi-pi+pi+pi- decays
Source: arXiv:1308.3189 source file (2013-09-02)
Supplement: Supplementary file 1 [file supplementary-app.tex]

\section{Supplementary material}

\subsection{Alternative partitions}

The \SCP distributions with alternative partitions are 
shown in \fig{fig:altBinningKKPiPi} for \DKKPiPi decays and \fig{fig:altBinningFourPi} for \DFourPi decays. 

The \SCP distributions with alternative partitions for the \DKThreePi control channel are shown in \fig{fig:altBinningKThreePi},
for combined magnet up and magnet down data.

\begin{figure}[htbp]
        \centering
     \subfloat{\label{fig:SCP:KKPiPi_16}%
       \includegraphics[width=0.495\textwidth]{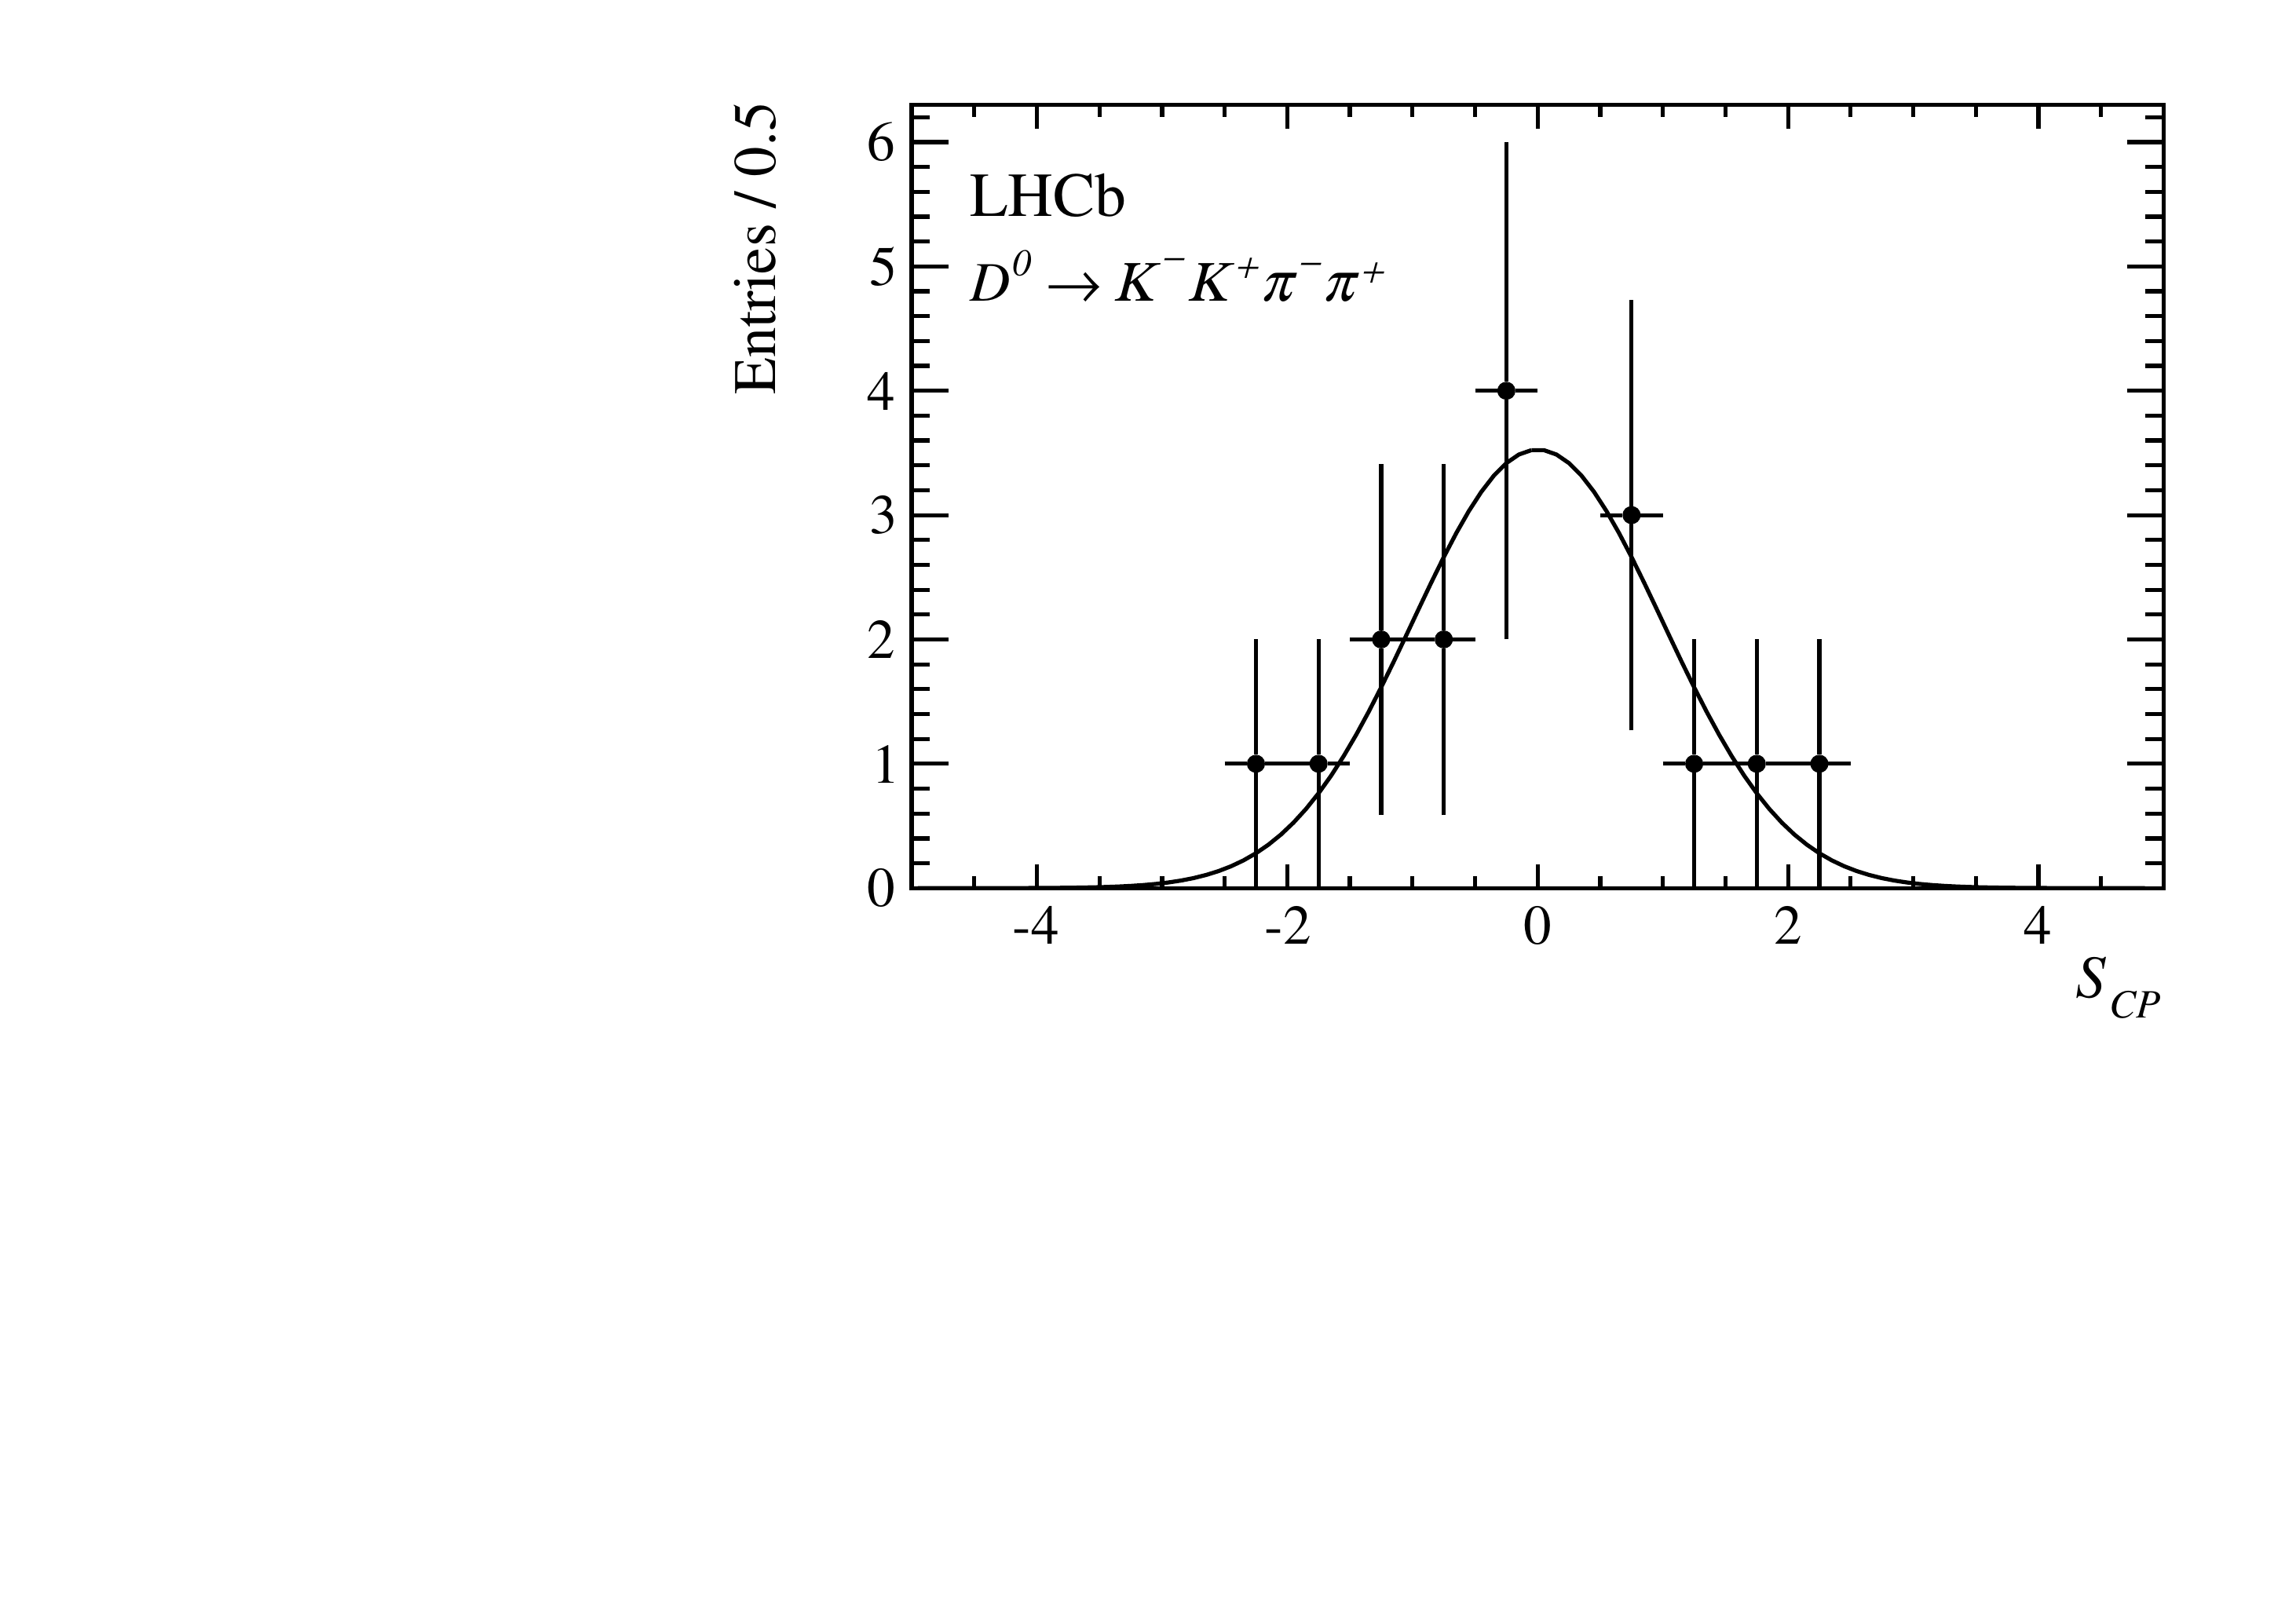}%
       \makebox[0cm][r]{\raisebox{0.19\textheight}[0cm]{\protect\subref{fig:SCP:KKPiPi_16}}\hspace{0.04\textwidth}}
     }%
     \subfloat{\label{fig:SCP:KKPiPi_64}%
       \includegraphics[width=0.495\textwidth]{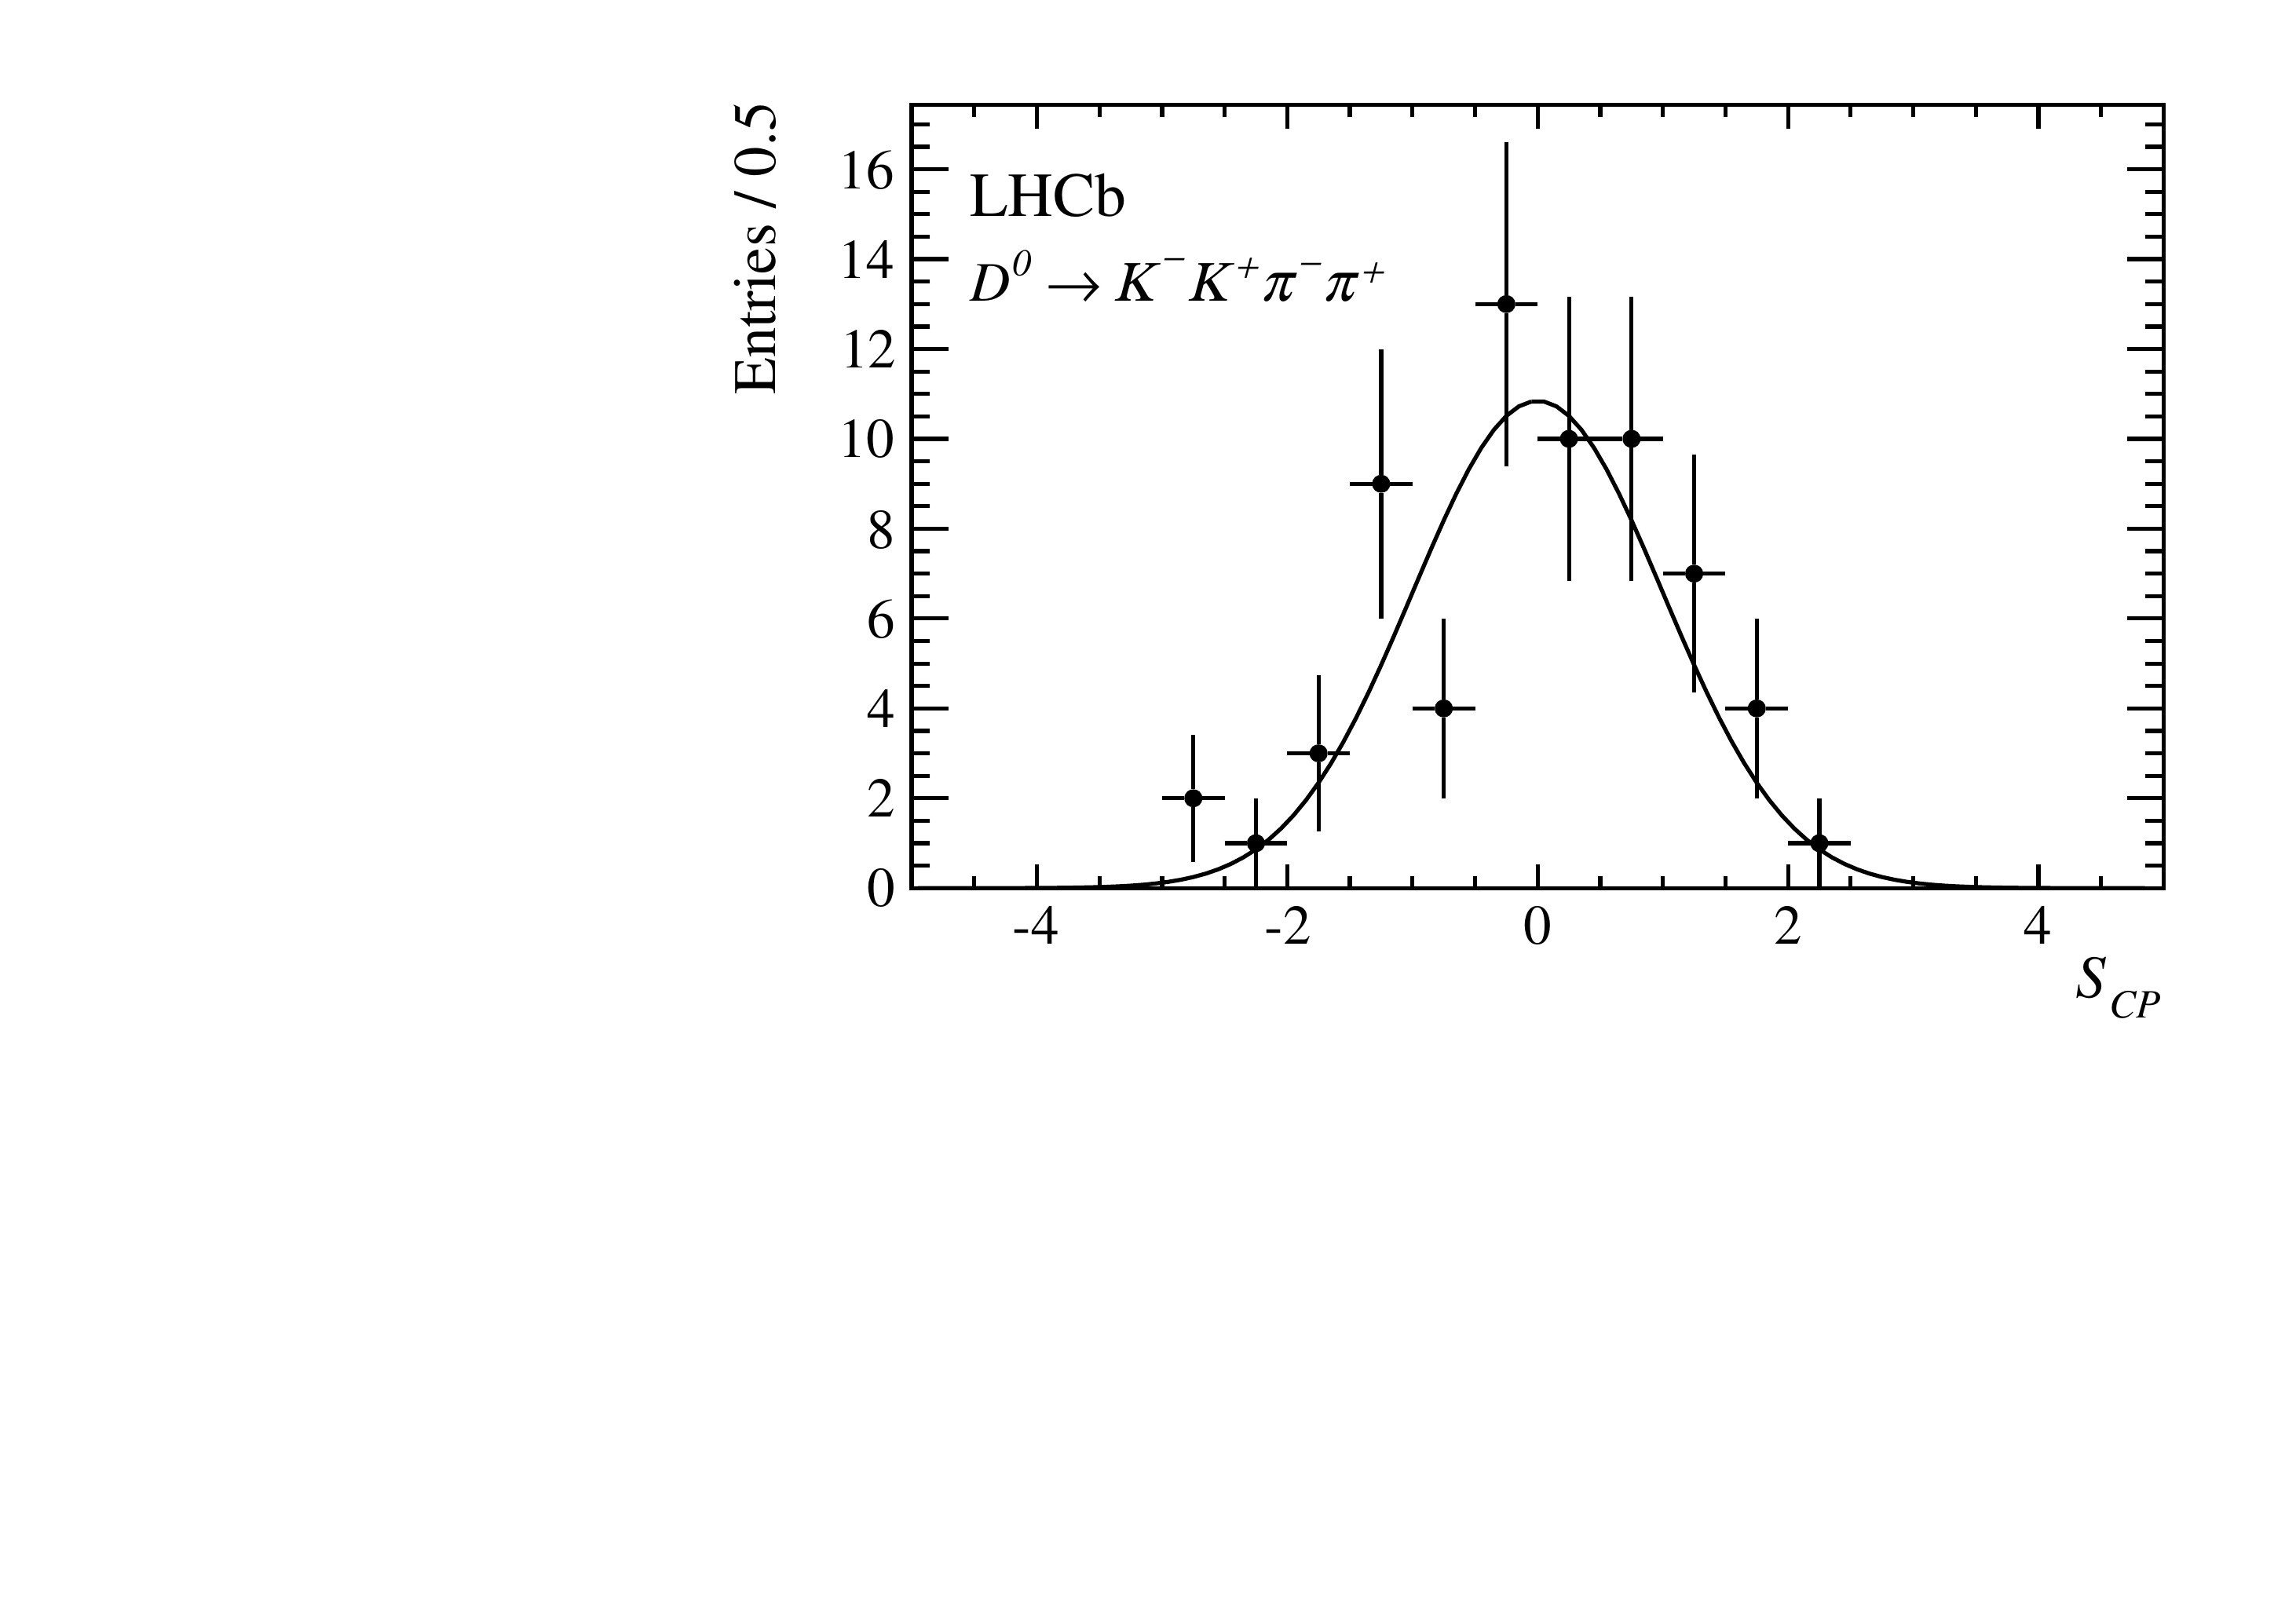}%
       \makebox[0cm][r]{\raisebox{0.19\textheight}[0cm]{\protect\subref{fig:SCP:KKPiPi_64}}\hspace{0.04\textwidth}}
     }%
                \caption{\small Distribution of \SCP for \DKKPiPi decays with \protect\subref{fig:SCP:KKPiPi_16} 16 bins and \protect\subref{fig:SCP:KKPiPi_64} 64 bins. The points show the data distribution and the solid line is a reference Gaussian distribution corresponding to the no CPV hypothesis.\label{fig:altBinningKKPiPi}}
\end{figure}

\begin{figure}[htbp]
        \centering
     \subfloat{\label{fig:SCP:FourPi_64}%
       \includegraphics[width=0.495\textwidth]{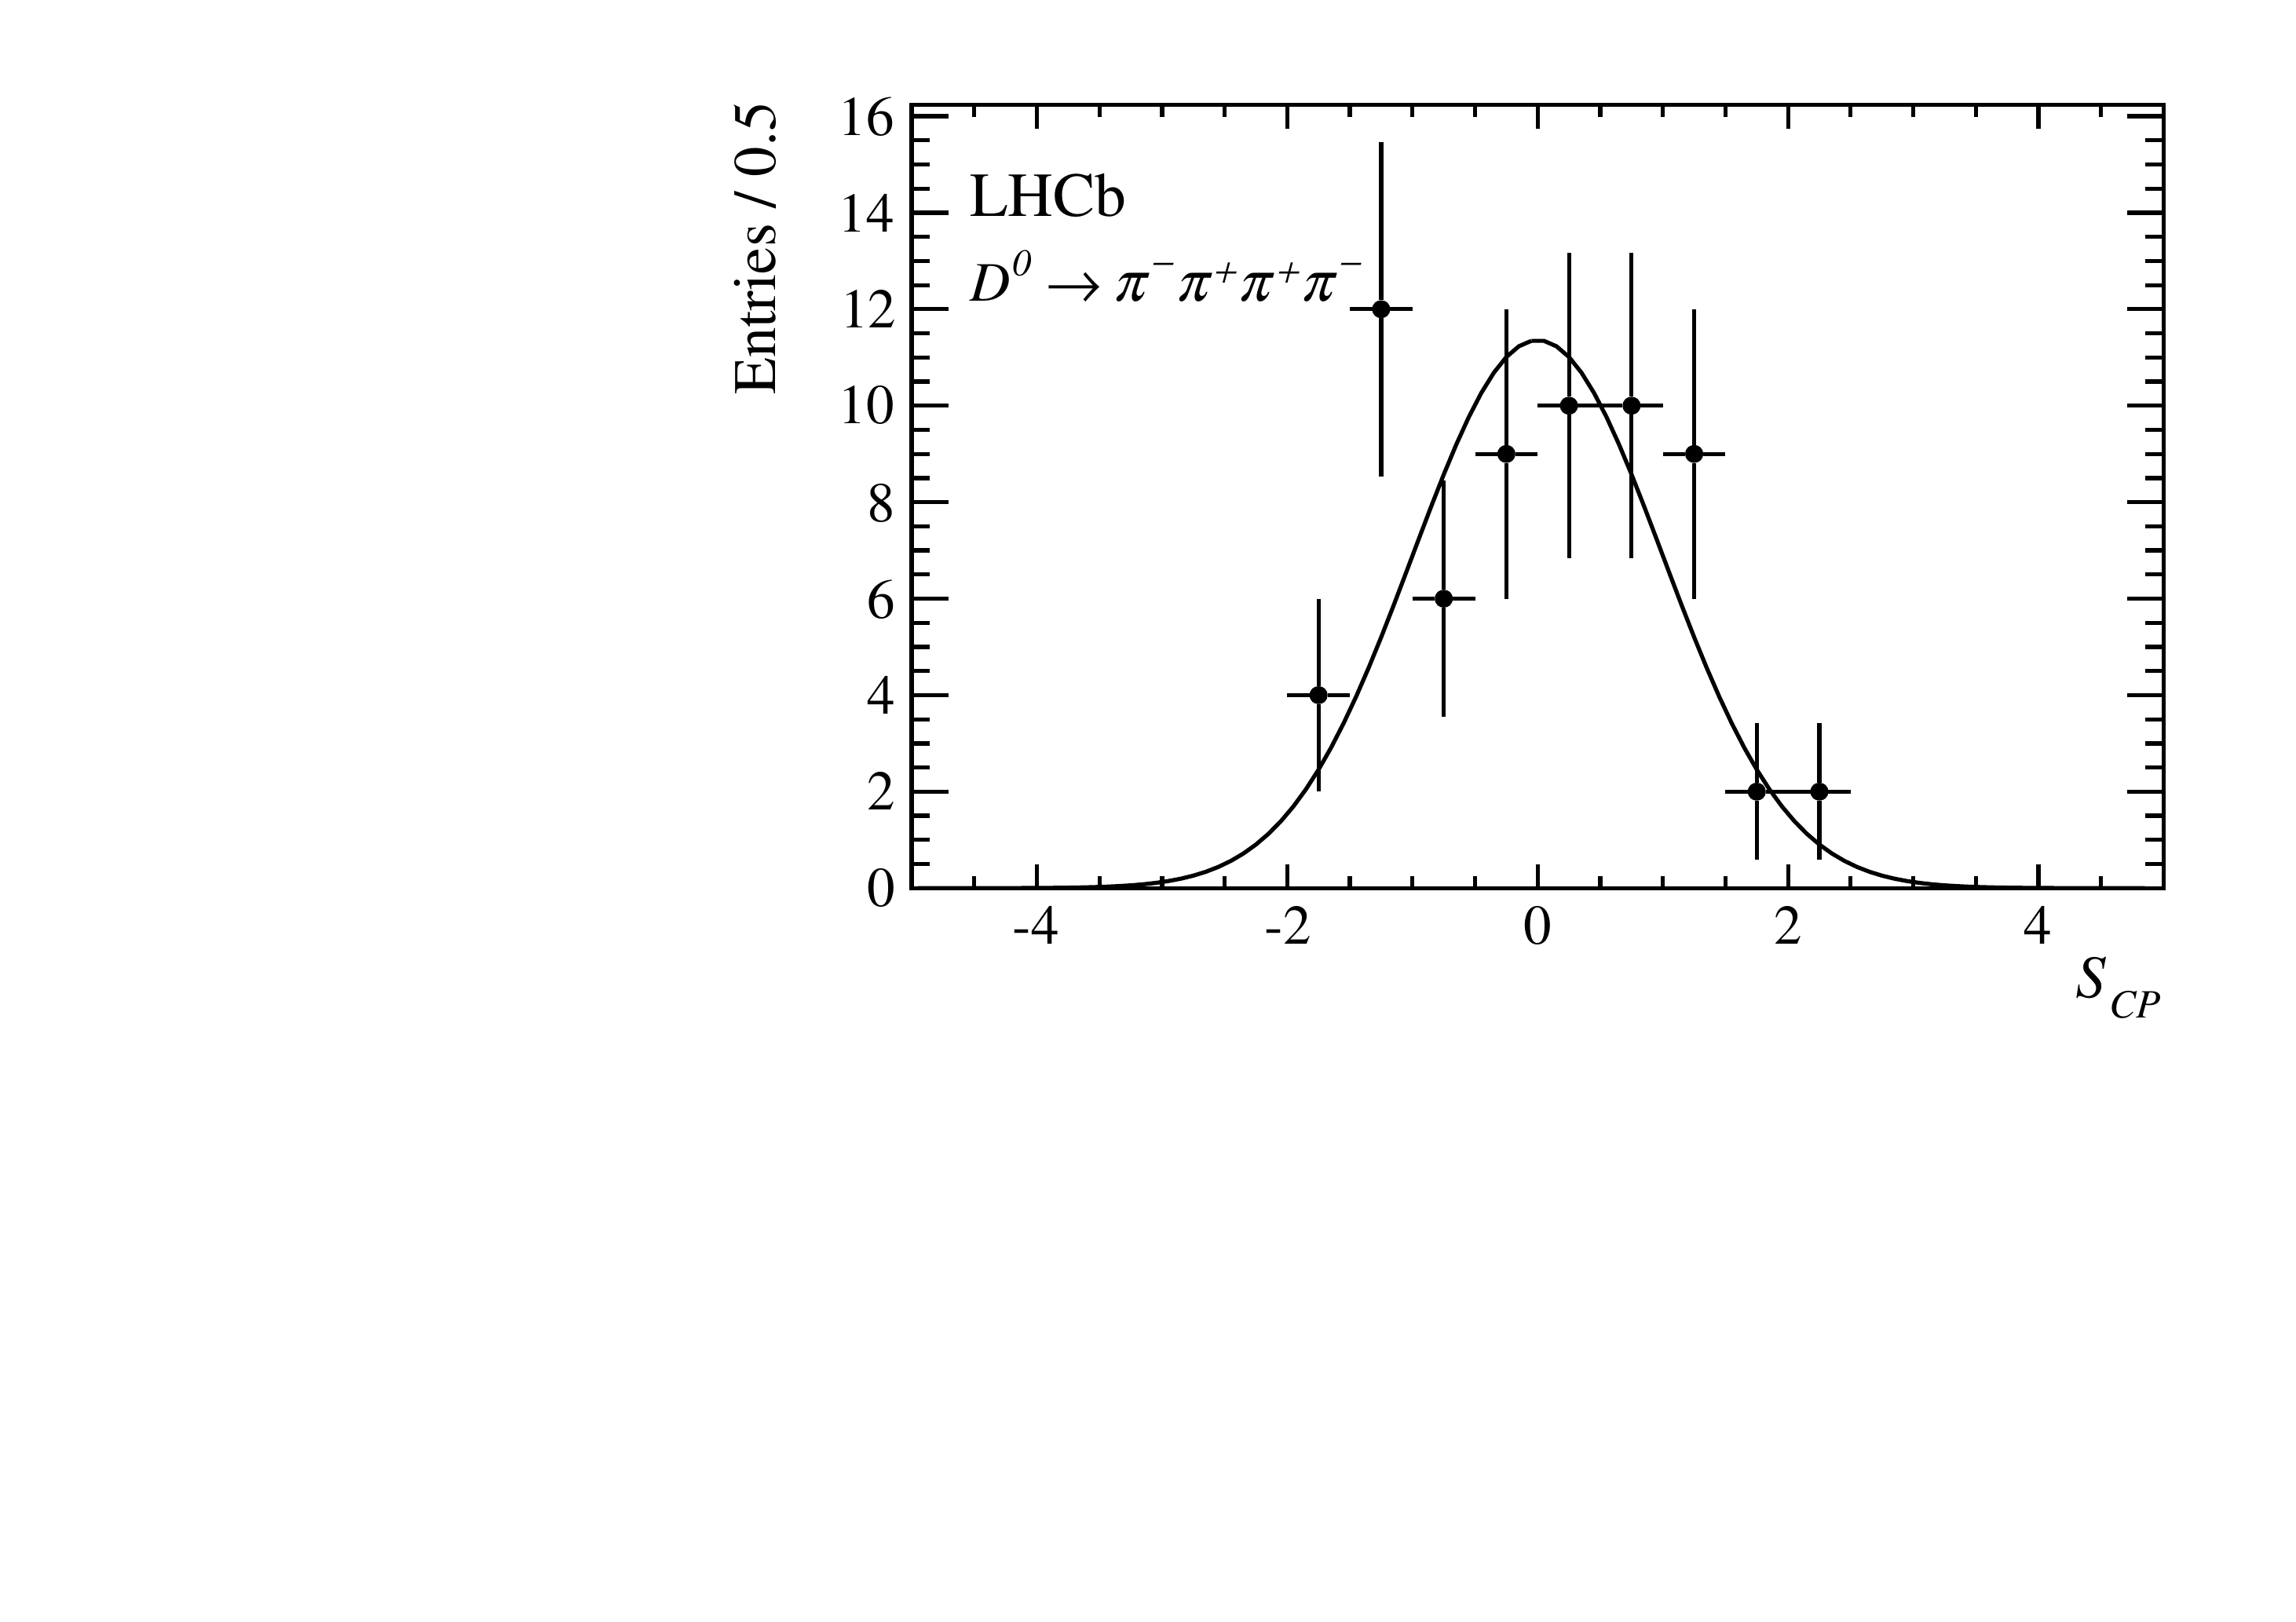}%
       \makebox[0cm][r]{\raisebox{0.19\textheight}[0cm]{\protect\subref{fig:SCP:FourPi_64}}\hspace{0.04\textwidth}}
     }%
     \subfloat{\label{fig:SCP:FourPi_256}%
       \includegraphics[width=0.495\textwidth]{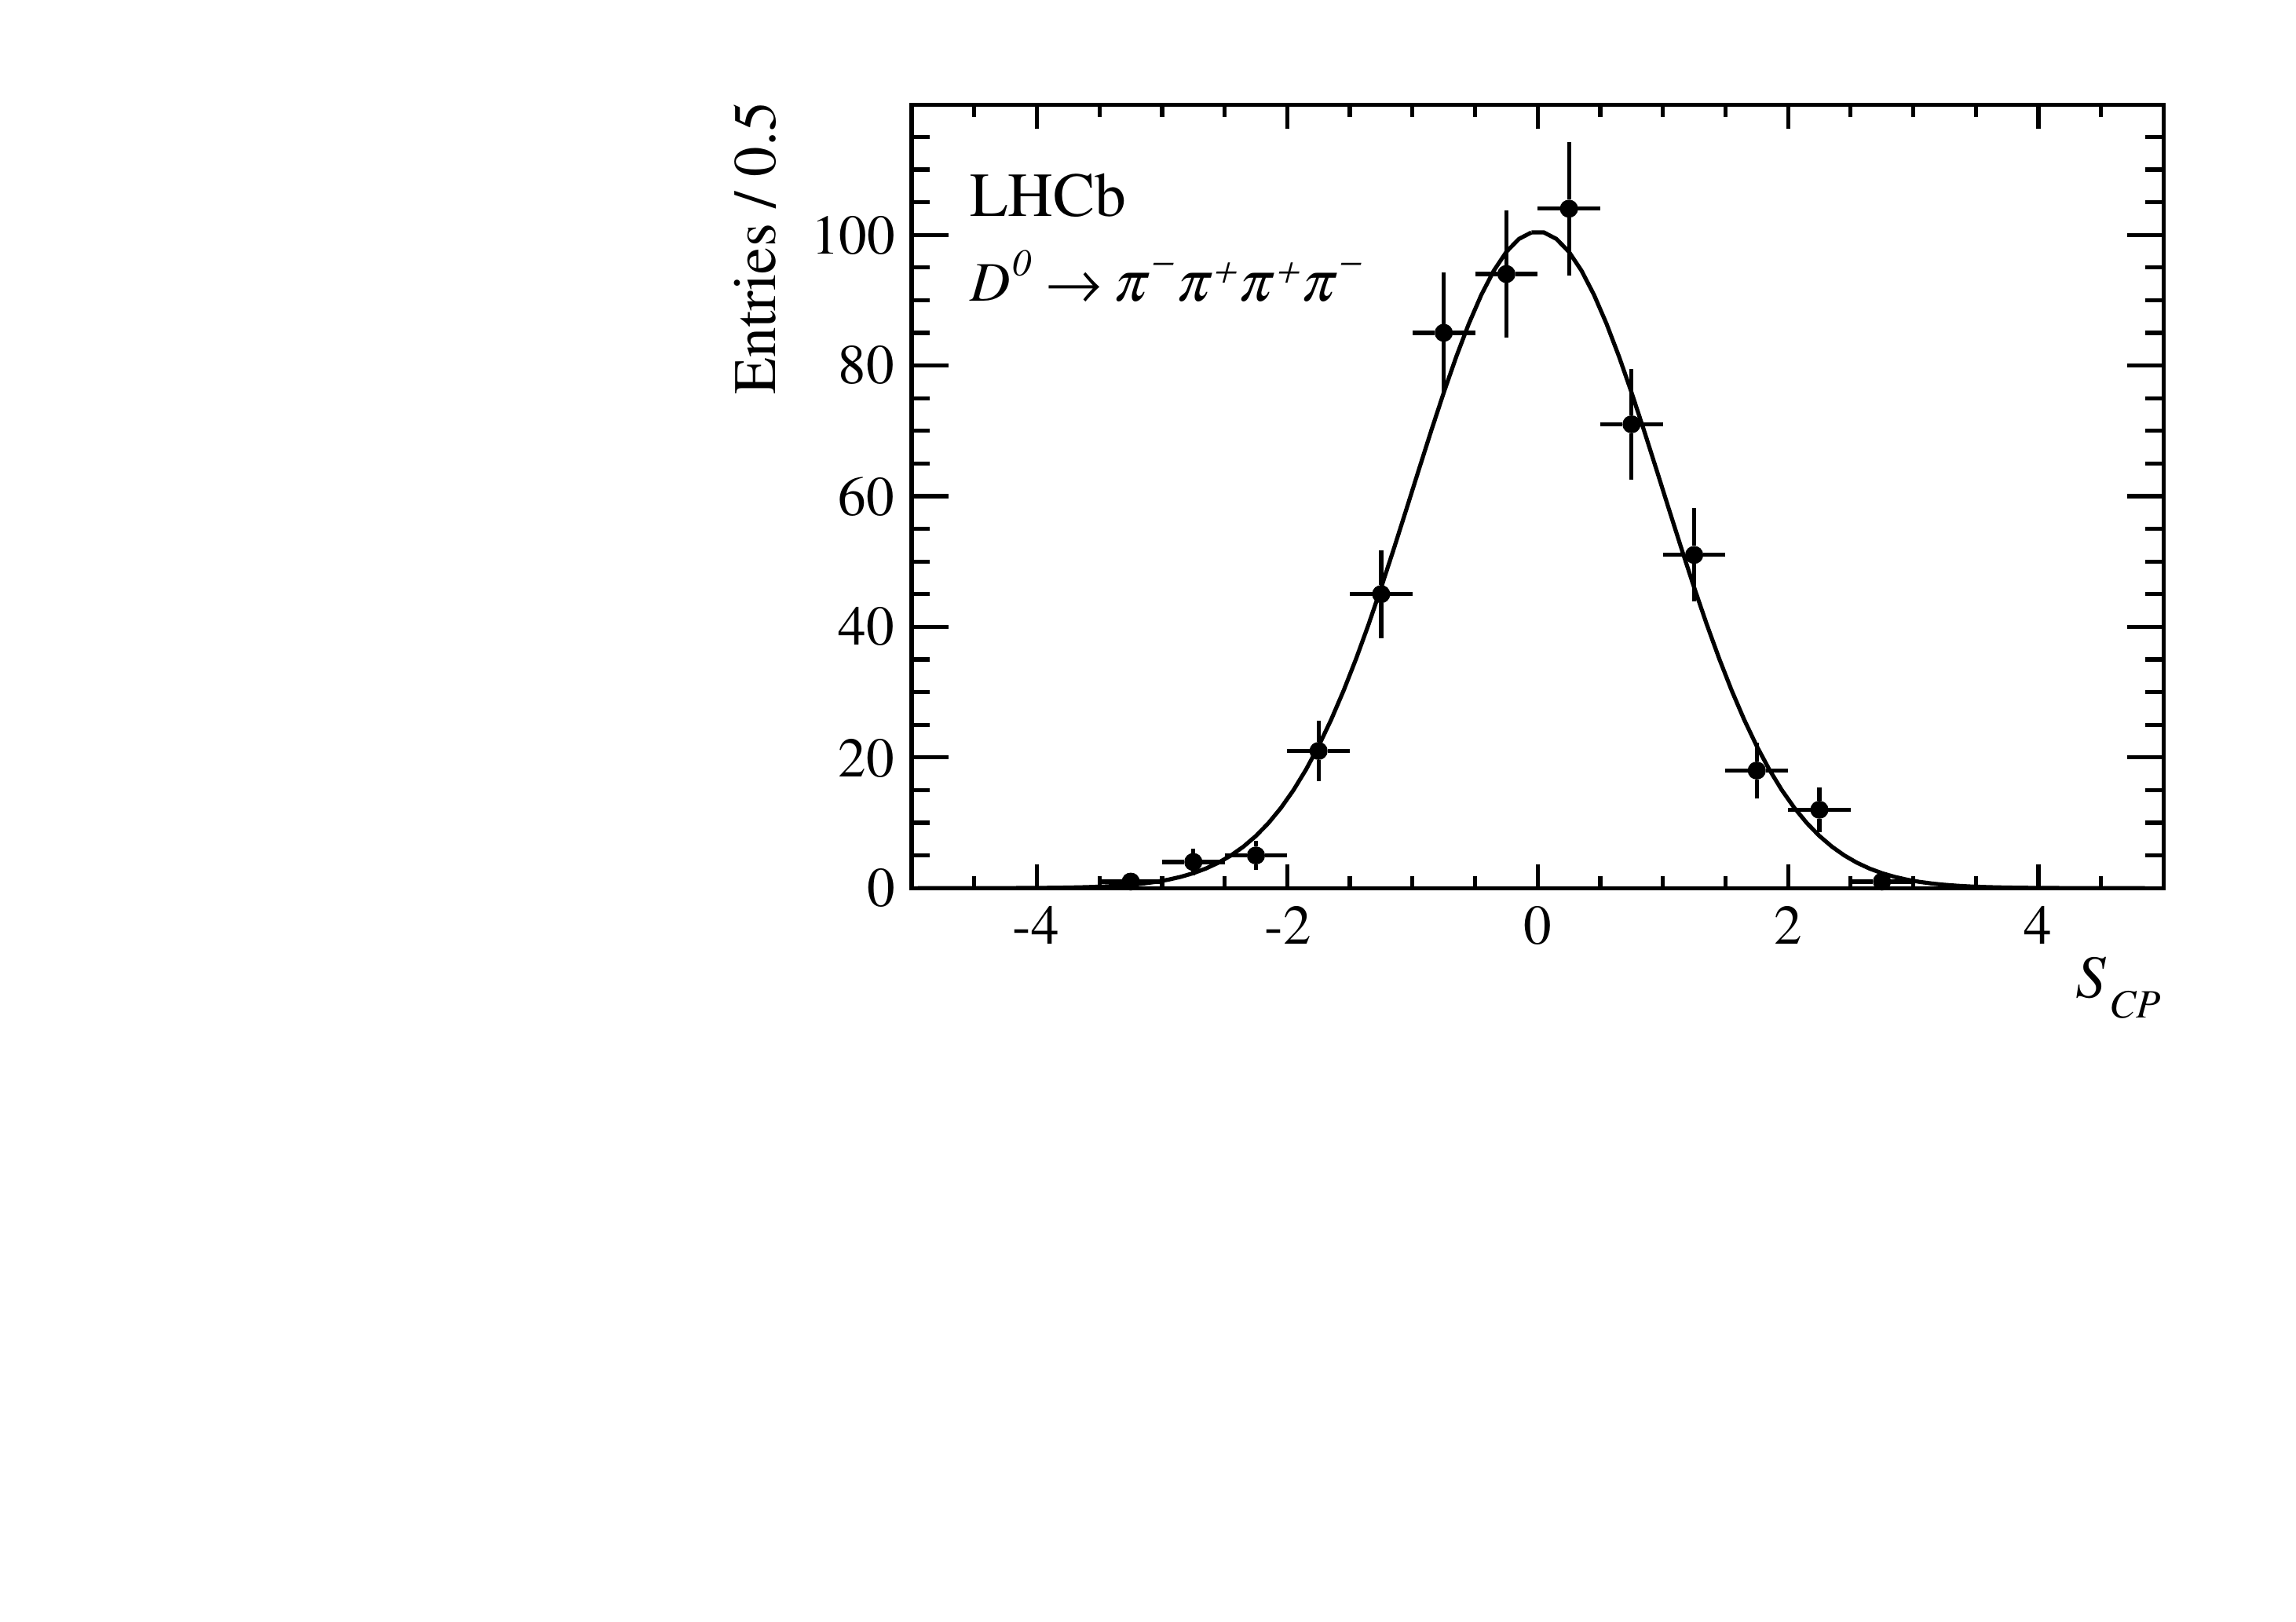}%
       \makebox[0cm][r]{\raisebox{0.19\textheight}[0cm]{\protect\subref{fig:SCP:FourPi_256}}\hspace{0.04\textwidth}}
     }%

                \caption{\small Distribution of \SCP for \DFourPi decays with \protect\subref{fig:SCP:FourPi_64} 64 bins and  \protect\subref{fig:SCP:FourPi_256} 256 bins. The points show the data distribution and the solid line is a reference Gaussian distribution corresponding to the no CPV hypothesis.\label{fig:altBinningFourPi}}
\end{figure}

\begin{figure}[htbp]
        \centering
     \subfloat{\label{fig:SCP:KThreePi_16}%
       \includegraphics[width=0.495\textwidth]{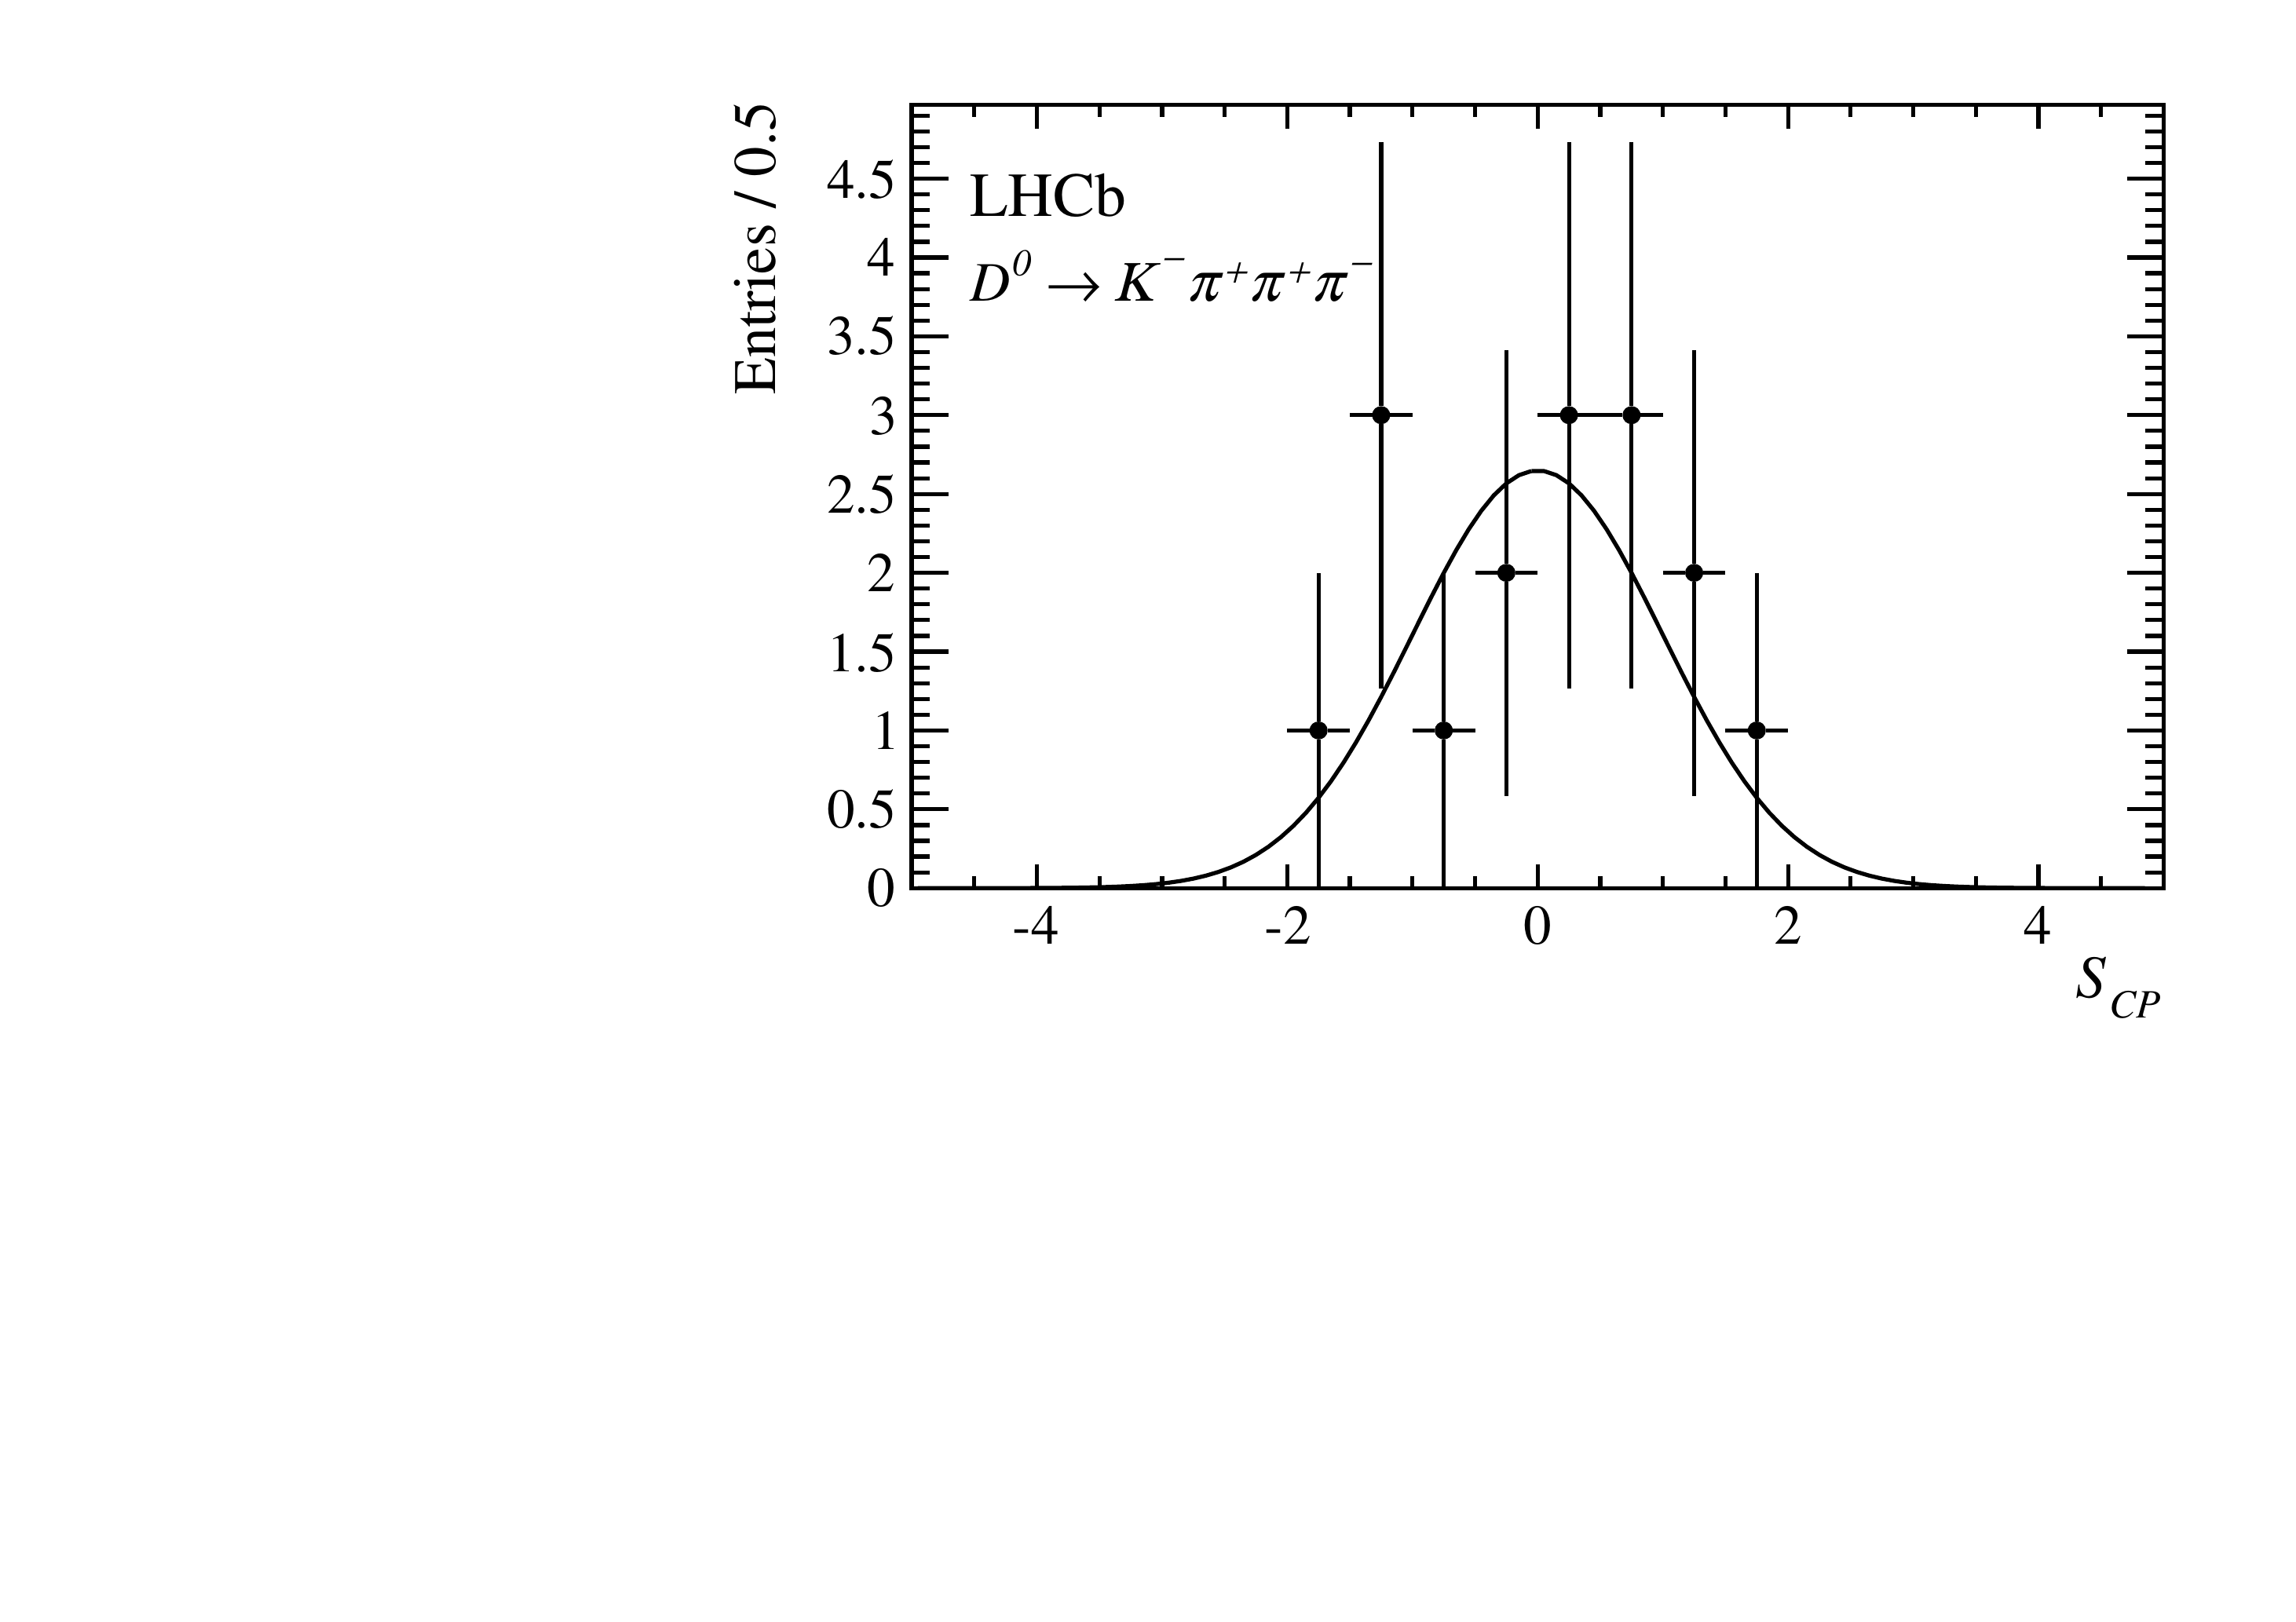}%
       \makebox[0cm][r]{\raisebox{0.19\textheight}[0cm]{\protect\subref{fig:SCP:KThreePi_16}}\hspace{0.04\textwidth}}
     }%
        \subfloat{\label{fig:SCP:KThreePi_1024}%
       \includegraphics[width=0.495\textwidth]{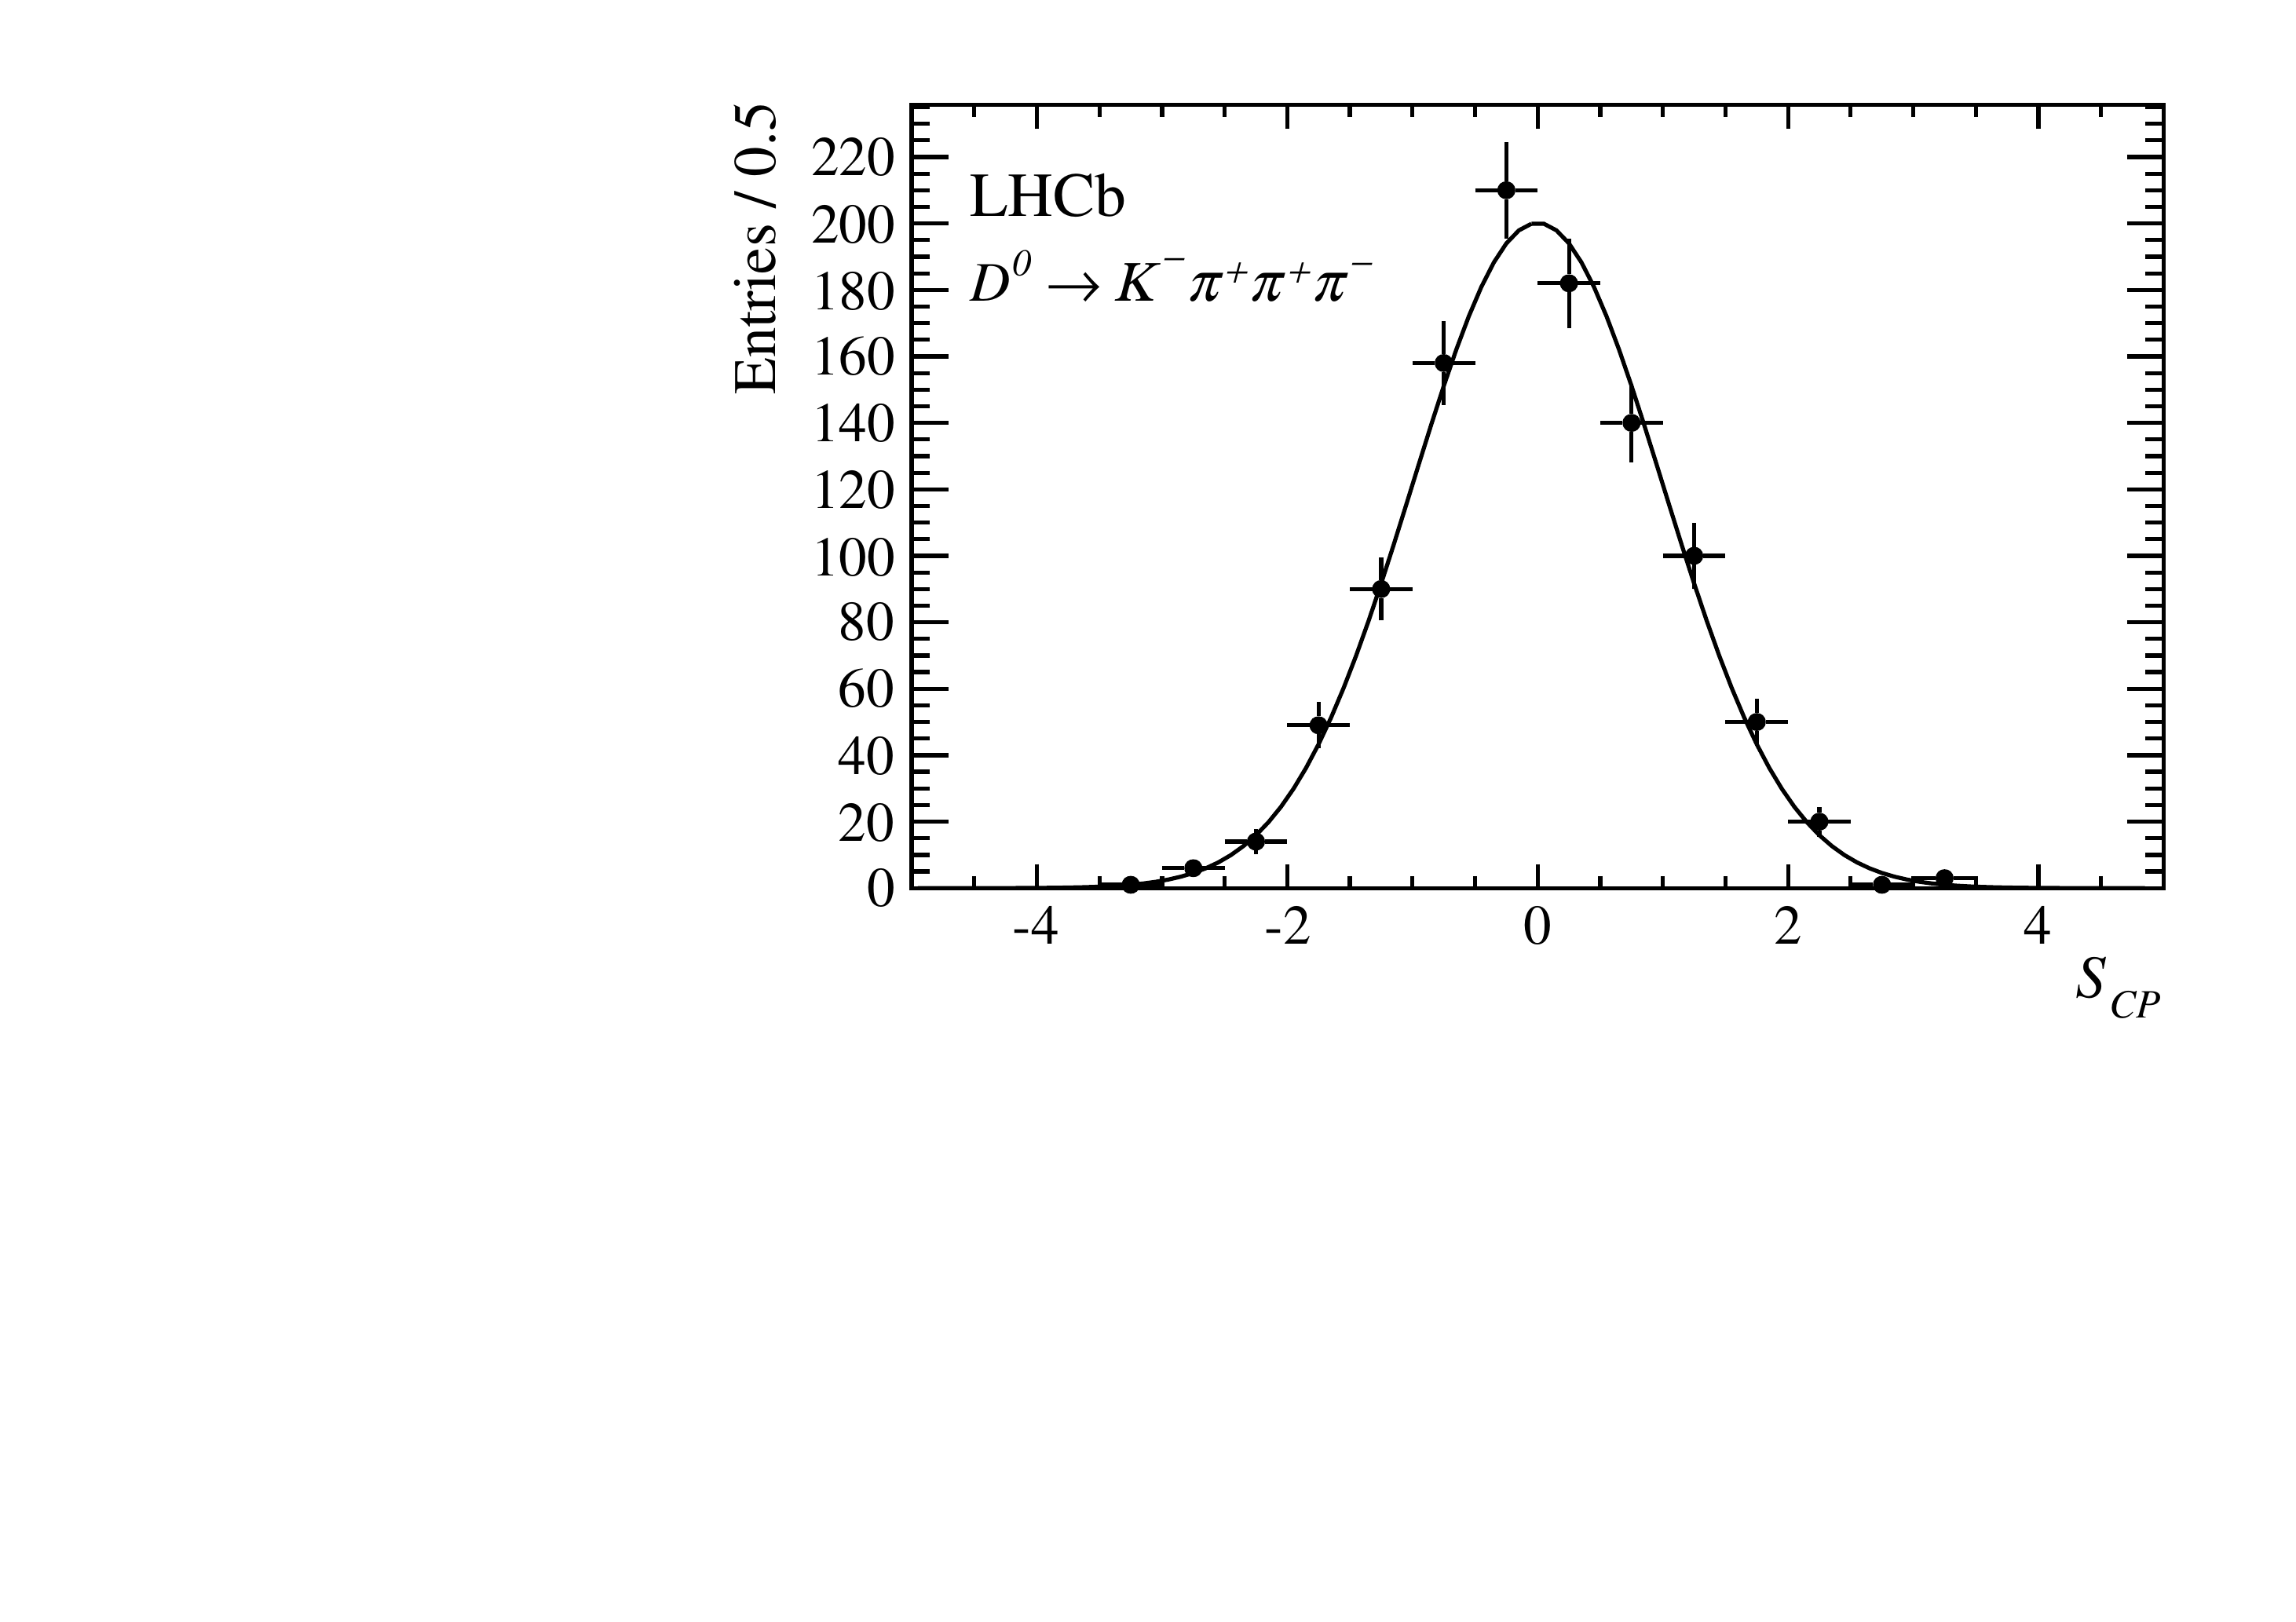}%
       \makebox[0cm][r]{\raisebox{0.19\textheight}[0cm]{\protect\subref{fig:SCP:KThreePi_1024}}\hspace{0.04\textwidth}}
     }%
   \caption{\small Distribution of \SCP for \DKThreePi decays with \protect\subref{fig:SCP:KThreePi_16} 16 bins and \protect\subref{fig:SCP:KThreePi_1024} 1024 bins. The points show the data distribution and the solid line is a reference Gaussian distribution corresponding to the no CPV hypothesis.\label{fig:altBinningKThreePi}}
\end{figure}

\subsection{Bin definitions}

The phase-space partitions for \DKKPiPi and \DFourPi decays are defined in 
terms of five invariant mass-squared combinations of the \Dz meson decay products. 
The definitions of default partitions in terms of these five variables are shown along with the \SCP value for each corresponding bin for \DKKPiPi decays 
and \DFourPi decays in  \fig{fig:KKPiPiBinning}  and \fig{fig:FourPiBinning}, respectively. 

\begin{figure}[htbp]
        \centering
     \subfloat{\label{fig:KKPiPiBinning1}%
       \includegraphics[width=0.705\textwidth]{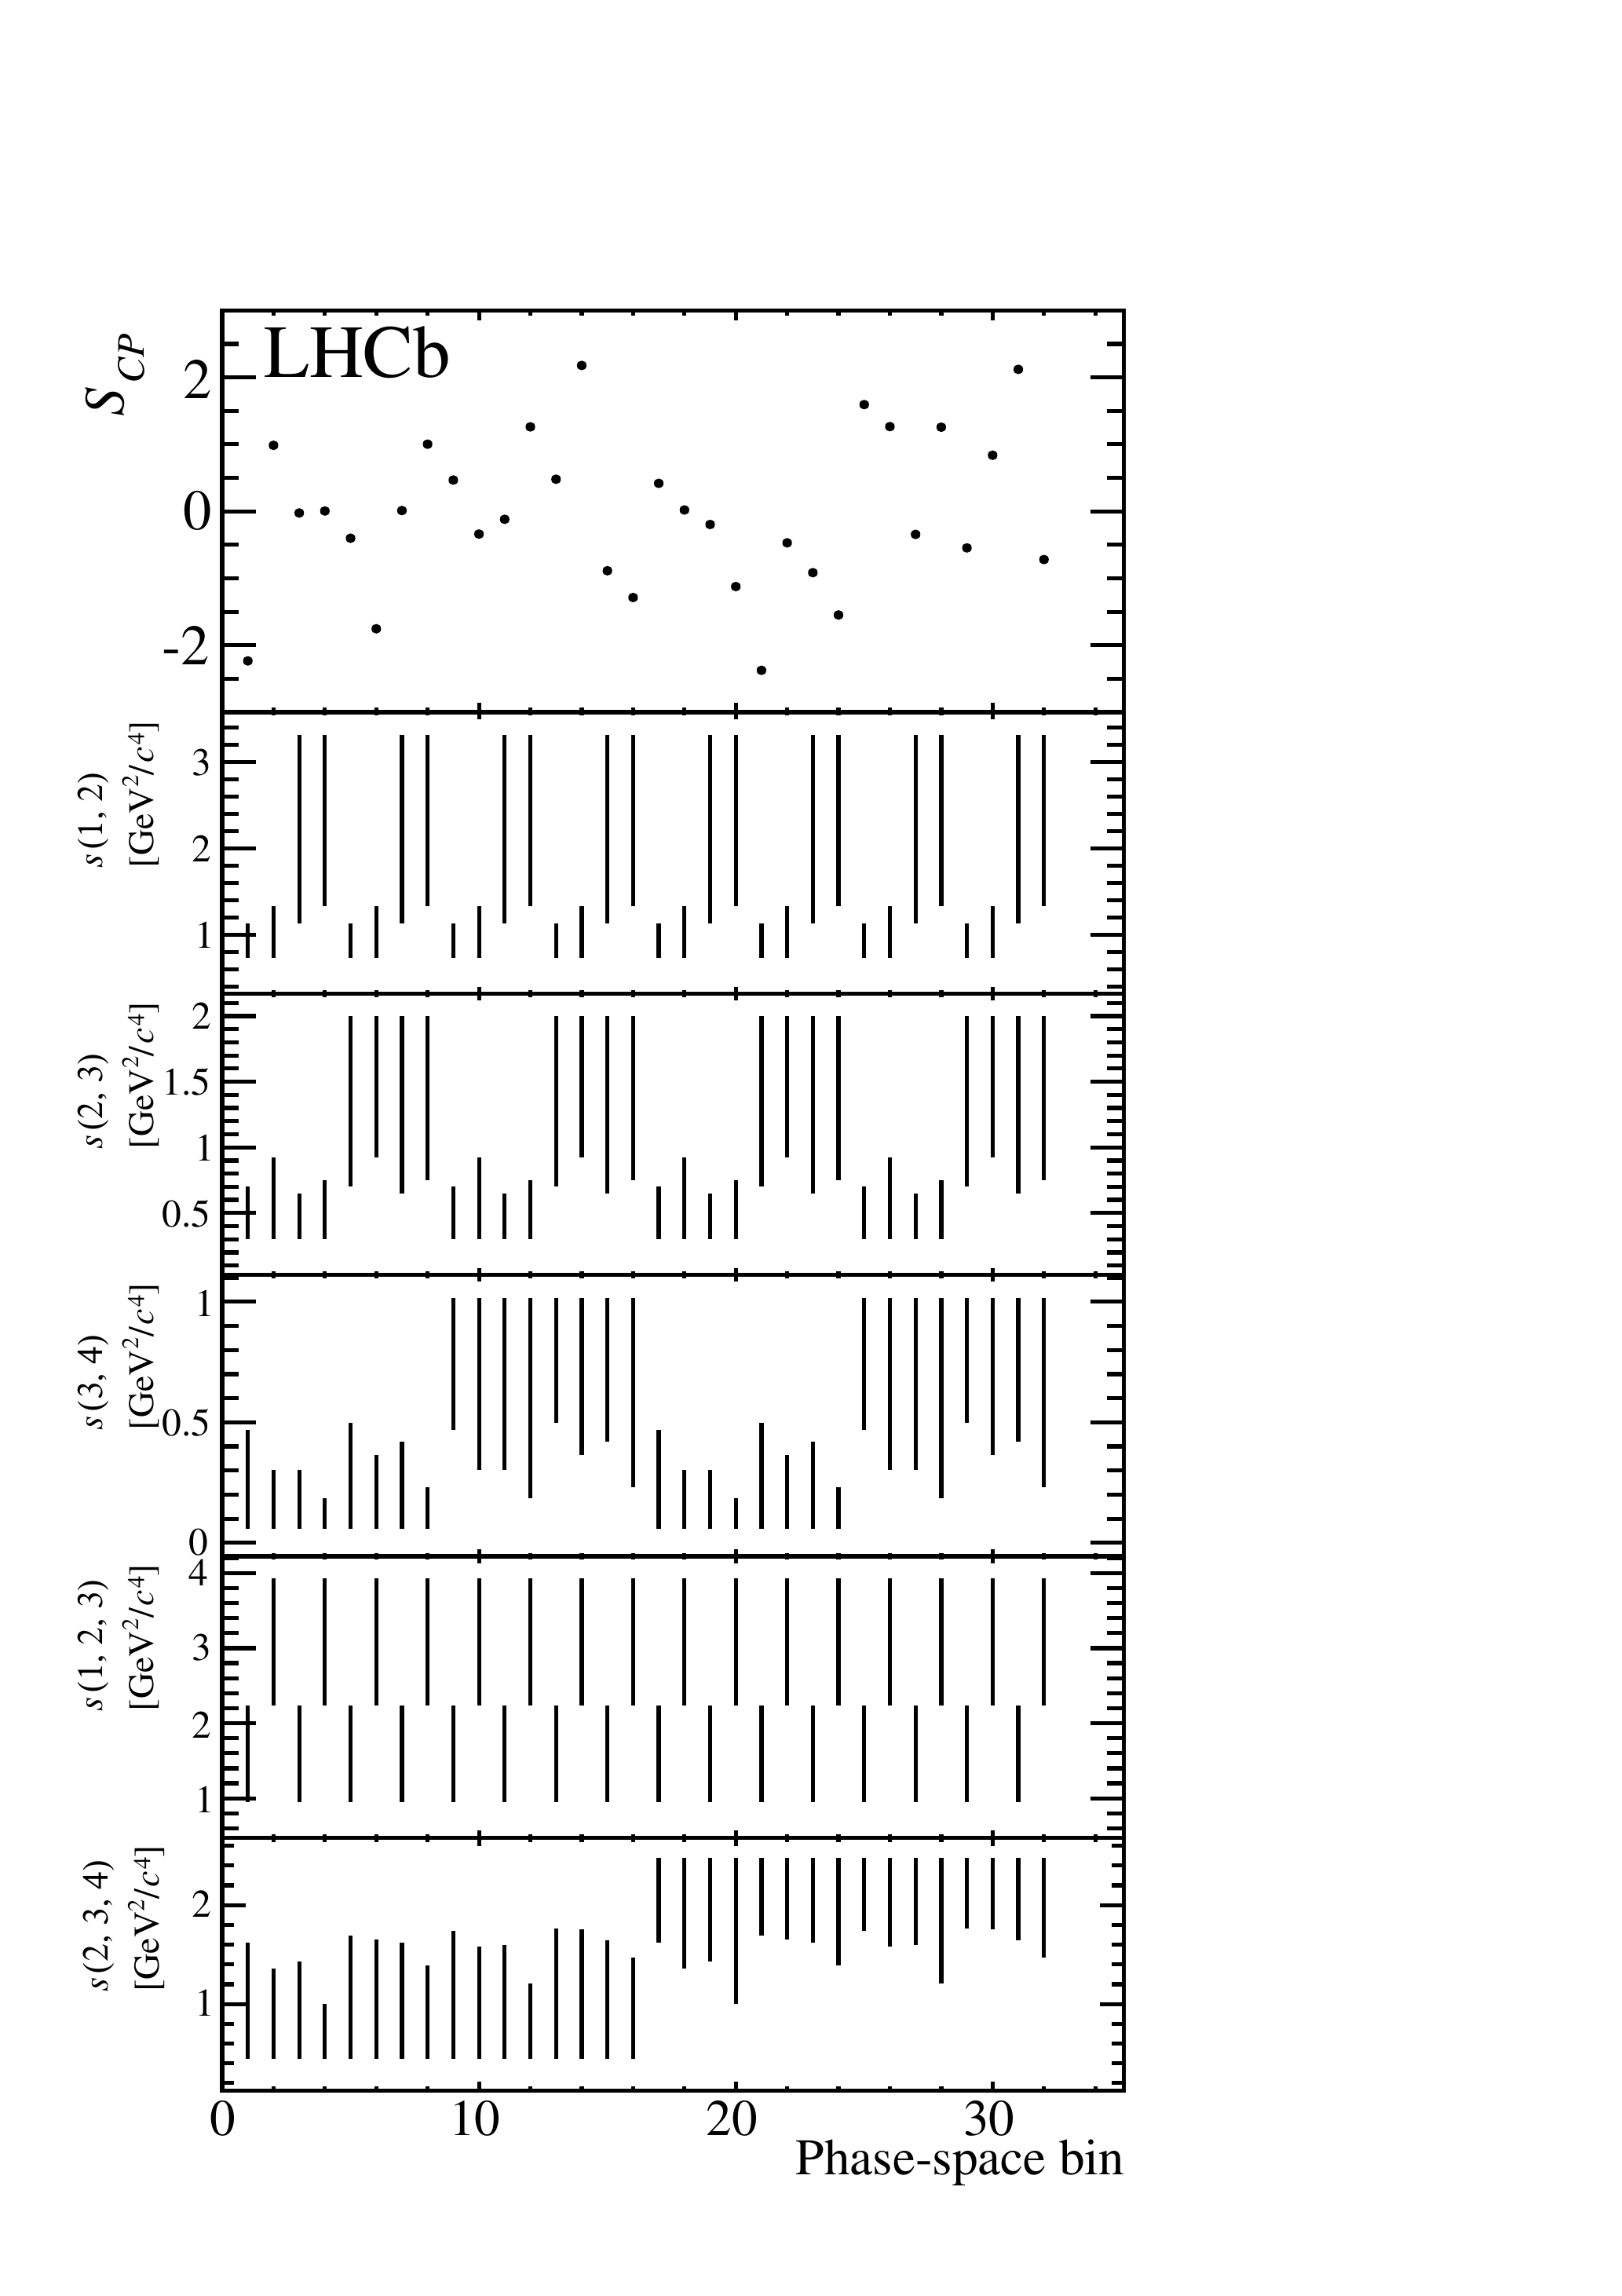}%
}
                \caption{\small Definitions of the default partition of 32 bins across the five-dimensional phase space of the \DKKPiPi decay. 
The vertical lines show the range covered in the given invariant mass-squared combination in units of \gevgevcccc. The invariant mass-squared combinations \invariantMassCombs correspond to \invariantMassCombsKKPiPi, respectively. The markers on the first plot show the value of \SCP for each corresponding bin. 
\label{fig:KKPiPiBinning}}
\end{figure}

\begin{figure}[htbp]
        \centering
     \subfloat{\label{fig:FourPiBinning1}%
       \includegraphics[width=0.705\textwidth]{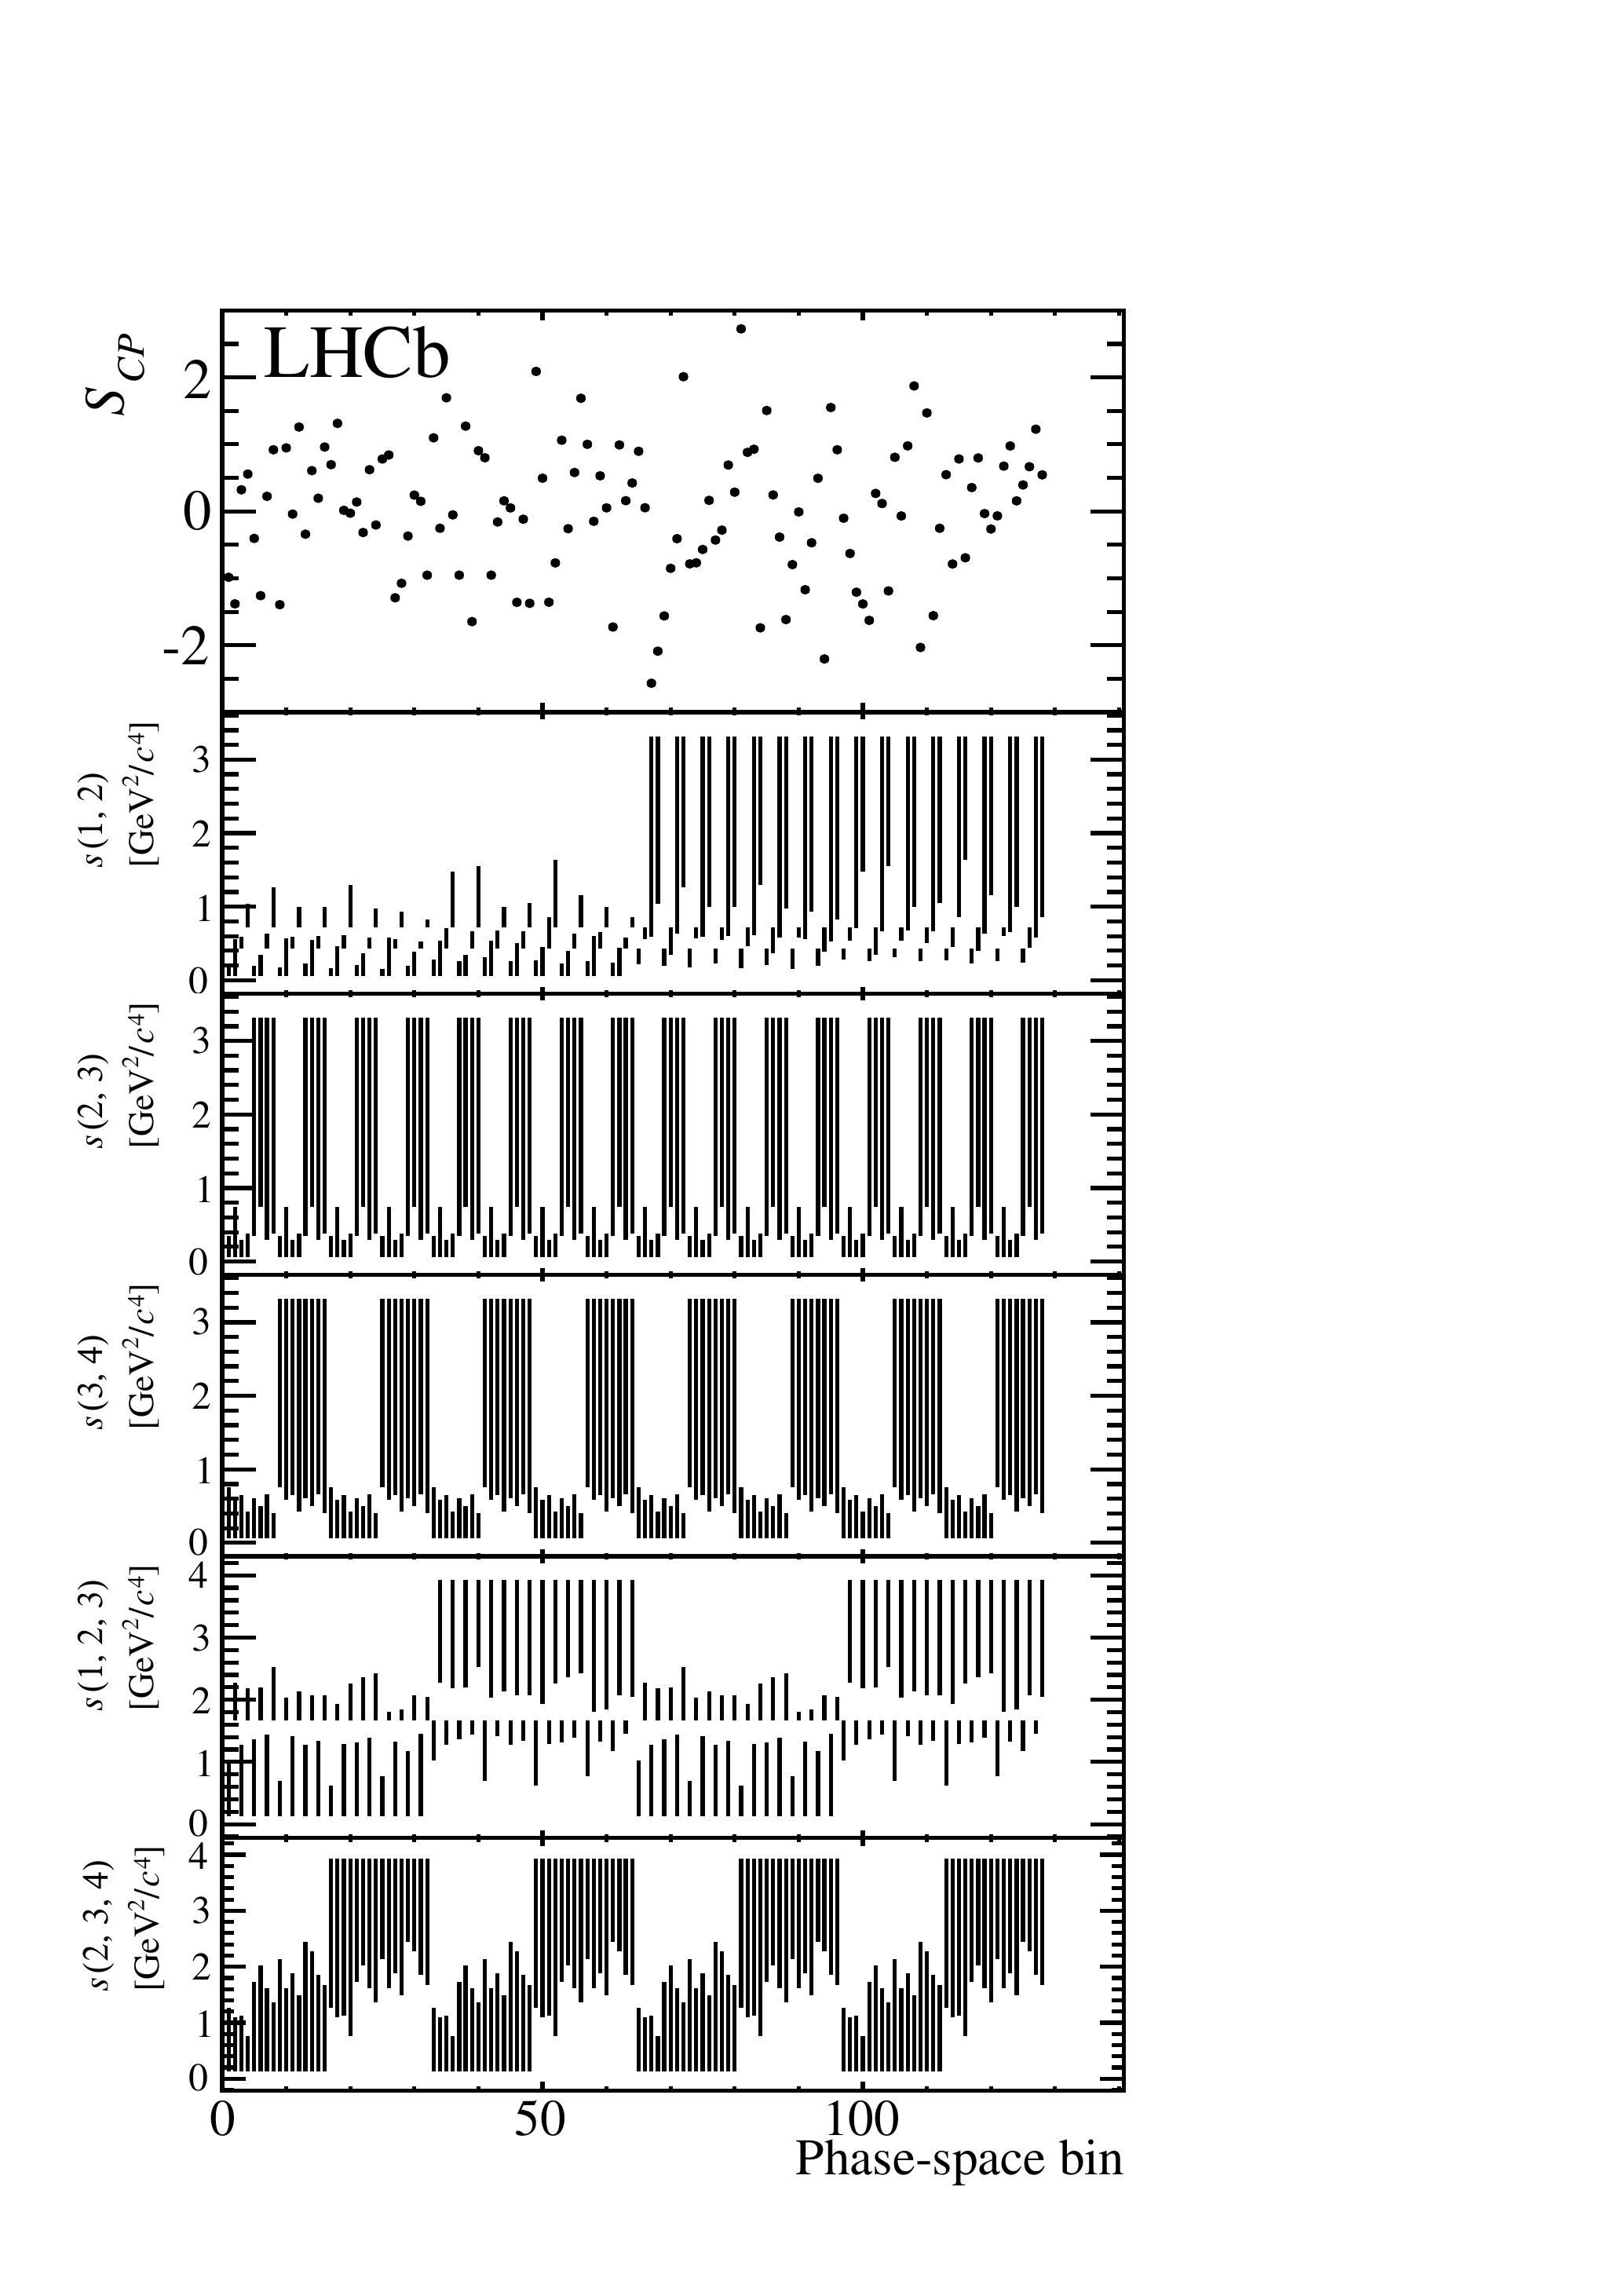}%
}
                \caption{\small Definitions of the default partition of 128 bins across the five-dimensional phase space of the \DFourPi decay. 
The vertical lines show the range covered in the given invariant mass-squared combination in units of \gevgevcccc. The invariant mass-squared combinations \invariantMassCombs correspond to \invariantMassCombsFourPi, respectively. The markers on the first plot show the value of \SCP for each corresponding bin. 
\label{fig:FourPiBinning}}
\end{figure}
